# Supplementary material for: Genetic algorithms for multi-omic feature selection: a comparative study in cancer survival analysis
Source: arXiv:2604.00065 source file (2026-03-31)
Supplement: Supplementary file 1 [file doc_setup_supplementary.tex]

\documentclass[paper=a4,fontsize=8pt]{scrartcl}
  \addtokomafont{sectioning}{\rmfamily}
  \addtokomafont{caption}{\rmfamily}
  \addtokomafont{caption}{\footnotesize}
\usepackage{float}
\usepackage{graphicx} % Required for inserting images
\usepackage[export]{adjustbox}
\usepackage[margin={1.5cm,1.5cm}]{geometry}
\usepackage{relsize}
\usepackage{doi}
\usepackage{xcolor}
\usepackage{authblk}
\hypersetup{nolinks=true}
\setlength\columnsep{0.5cm}
\usepackage{natbib}
\bibliographystyle{abbrvnat}
\setcitestyle{authoryear,round,aysep={}}

\setcounter{figure}{0}

\setcounter{table}{0}

\usepackage{xr}

\usepackage{multicol}

\let\OLDthebibliography\thebibliography
\renewcommand\thebibliography[1]{
  \OLDthebibliography{#1}
  \setlength{\parskip}{0pt}
  \setlength{\itemsep}{0pt plus 0.3ex}
}

\usepackage{abstract}
\setlength{\absleftindent}{0mm}
\setlength{\absrightindent}{0mm}

\usepackage{algorithm}% http://ctan.org/pkg/algorithms
\usepackage{algpseudocode}% http://ctan.org/pkg/algorithmicx

\graphicspath{{Fig/}}

\usepackage{booktabs}
